# Supplementary material for: Optimal Policies Tend to Seek Power
Source: arXiv:1912.01683 source file (2023-01-28)
Supplement: Supplementary file 1 [file detour-src.tex]

\documentclass{standalone}
\usepackage{main-tex/preamble}
\input{main-tex/macros.tex}
\begin{document}
      \begin{tikzpicture}[> = latex, % arrow head style
            shorten > = 1pt, % don't touch arrow head to node
            auto,
            node distance = 1.3cm, % distance between nodes
            %ultra thick, % line style
            line width = 0.08 em
        ]

        %nodes
        \node[blue] (1) {$1$};
        \node[black] (2) [above of=1] {$2$};
        \node[black] (3) [right of=2] {$3$};
        \node[black] (4) [right of=3] {};
        \node[black] (5) [below right of=3] {};
        
        %arrows
        \path[->] (1) edge node[midway,left]{\texttt{N}} (2);
        \path[->] (1) edge node[near start, right=4pt]{\texttt{NE}}  (3);
        
        \arcHelp[-2.5pt][9pt]{N}{2};
        \path[->] (2) edge[color=gray] (3);
        
        \path[->] (3) edge (4);
        \path[->] (3) edge (5);
        
        \arcHelp[3.5pt]{NE}{4};
        \arcHelp[3pt][-.5pt]{SE}{5};
    \end{tikzpicture}
\end{document}
