# Supplementary material for: Optimal Policies Tend to Seek Power
Source: arXiv:1912.01683 source file (2023-01-28)
Supplement: Supplementary file 3 [file empower-weaker-src.tex]

\documentclass{standalone}
\usepackage{main-tex/preamble}
\input{main-tex/macros.tex}
\begin{document}
\begin{tikzpicture}[
            > = latex, % arrow head style
            shorten > = 1pt, % don't touch arrow head to node
            auto,
            node distance = 1.2cm, % distance between nodes
            %ultra thick, % line style
            line width = 0.08 em
        ]
        
        \node[blue] (1) {$3$};
        
        \node[black] (2) [below right of=1] {};
        \node[black] (3) [below left of=1] {};
        
        \node[red] (4) [below right of=2] {};
        \node[red] (5) [left of=4] {};
        \node[red] (7) [below left of=3] {};
        \node[red] (6) [right of=7] {};
        
        \path[->] (1) edge (2);
        \path[->] (1) edge (3);
        
        \path[->] (2) edge (4);
        \path[->] (2) edge (5);
        \path[->] (3) edge (6);
        \path[->] (3) edge (7);
        
        \arcHelp[0pt][0pt][.3cm]{S}{4};
        \arcHelp[0pt][0pt][.3cm]{S}{5};
        \arcHelp[0pt][0pt][.3cm]{S}{6};
        \arcHelp[0pt][0pt][.3cm]{S}{7};
    \end{tikzpicture}
\end{document}
