# Supplementary material for: Optimal Policies Tend to Seek Power
Source: arXiv:1912.01683 source file (2023-01-28)
Supplement: Supplementary file 4 [file fail-converge-src.tex]

\documentclass{standalone}
\usepackage{main-tex/preamble}
\input{main-tex/macros.tex}
\begin{document}
\begin{tikzpicture}[
            > = latex, % arrow head style
            shorten > = 1pt, % don't touch arrow head to node
            auto,
            node distance = 1.5cm, % distance between nodes
            %ultra thick, % line style
            line width = 0.08 em
        ]

        %nodes
        \node[blue] (1) {$1$};
        \node[black] (2) [right of=1] {$2$};
        
        %arrows
        \path[->] (1) edge [looseness=1, out=20, in=160] (2);
        \path[->] (2) edge [out=-160, in=-20] (1);
        
        \arcHelp{W}{1};
        \path[->] (2) edge [looseness=5, out=-45, in=45,color=white] (2);
        
     \end{tikzpicture}
 \end{document}
