# Supplementary material for: Optimal Policies Tend to Seek Power
Source: arXiv:1912.01683 source file (2023-01-28)
Supplement: Supplementary file 5 [file suboptimal-power-src.tex]

\documentclass{standalone}
\usepackage{main-tex/preamble}
\input{main-tex/macros.tex}
\begin{document}
\begin{tikzpicture}[
            > = latex, % arrow head style
            shorten > = 1pt, % don't touch arrow head to node
            auto,
            node distance = 1.5cm, % distance between nodes
            line width = 0.1 em
        ]

        \node[blue] (0) {$0$};
        
        % Right subgraph
        \node[black] (r) [right of=0] {$r$};
        \path[->] (0) edge (r) ;
        
        \node[black] (3) [above of=r] {$3$};
        \path[->] (r) edge (3);
        \arcHelp[-3.5pt][9pt][.3cm]{N}{3};
        
        \node[black] (4) [above right of=r] {$4$};
        \path[->] (r) edge (4);
        \arcHelp[2pt][3pt][.3cm]{NE}{4};
        
        \node[black] (5) [right of=r] {$5$};
        \path[->] (r) edge (5);
        \arcHelp[0pt][0pt][.3cm]{E}{5};
        
        % Left subgraph
        \node[black] (l) [left of=0] {$\ell$};
        \path[->] (0) edge (l);
                
        \node[black] (2) [above left of=l] {$2$};
        \path[->] (l) edge (2);
        \arcHelp[0pt][0pt][.3cm]{NW}{2};
        
        \node[black] (1) [left of=l] {$1$};
        \path[->] (l) edge (1);
        \arcHelp[0pt][0pt][.3cm]{W}{1};
     \end{tikzpicture}
 \end{document}
